# Supplementary material for: Hierarchical interpretations for neural network predictions
Source: arXiv:1806.05337 source file (2019-01-16)
Supplement: Supplementary file 1 [file supp_examples.pdf]

**SST top-predicted examples.** Here, the model used and figure produced correspond to Fig 2.

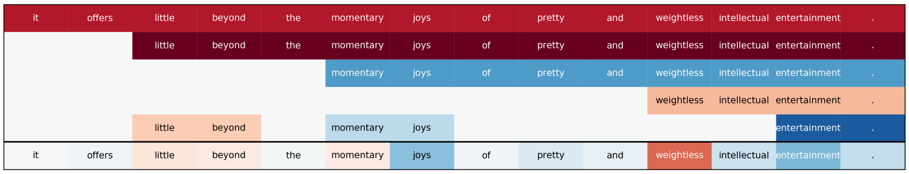


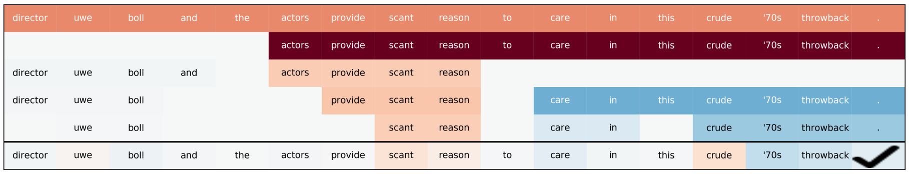


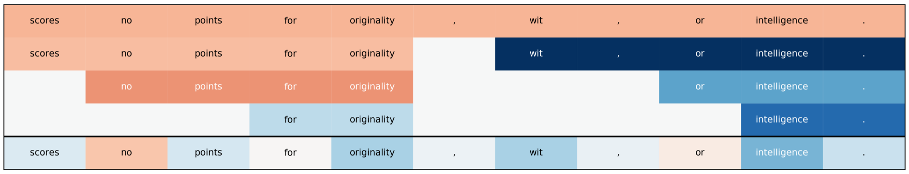


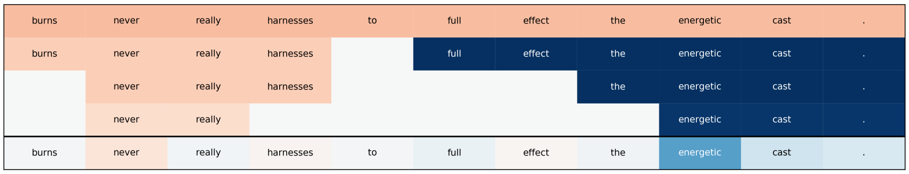


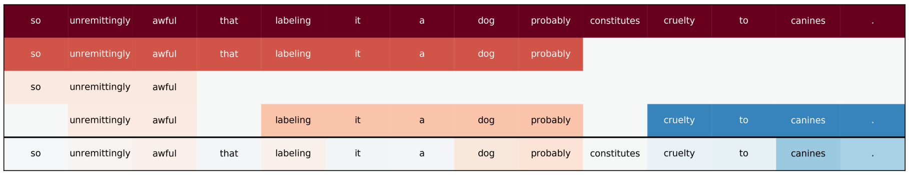


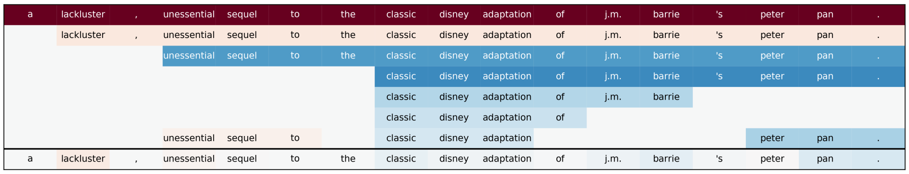

**SST lowest-predicted examples.** Here, the model used and figure produced correspond to Fig 2.

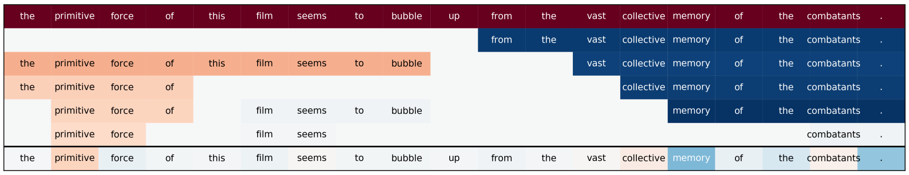


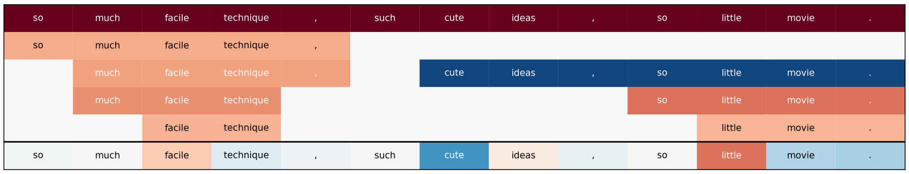


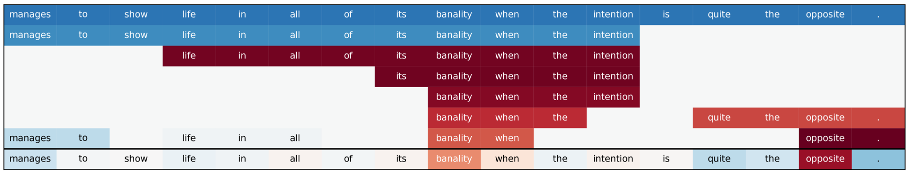


**MNIST top-predicted examples.** Here, the model used is the same as in Sec 4.3.2 and the interpretation of the figure produced is the same as in Fig 3.

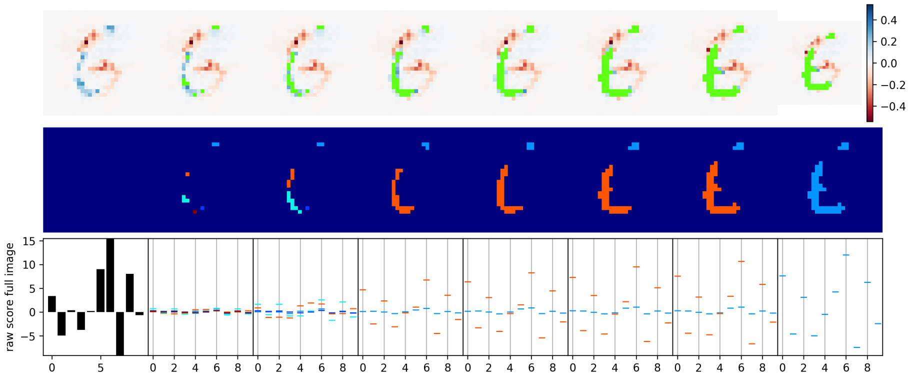

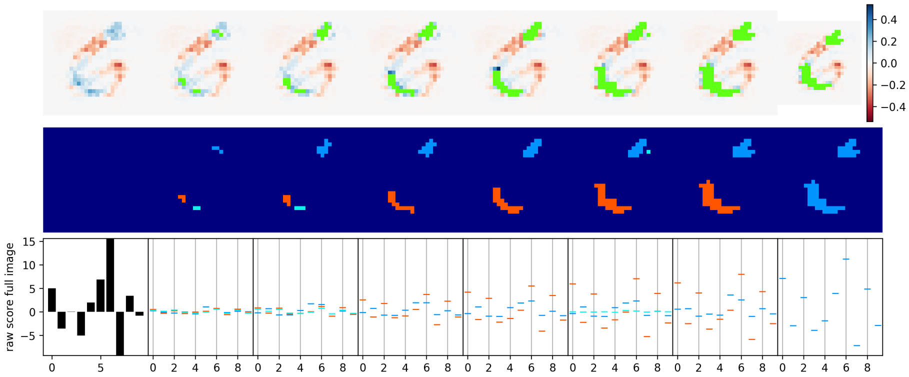
raw score full image

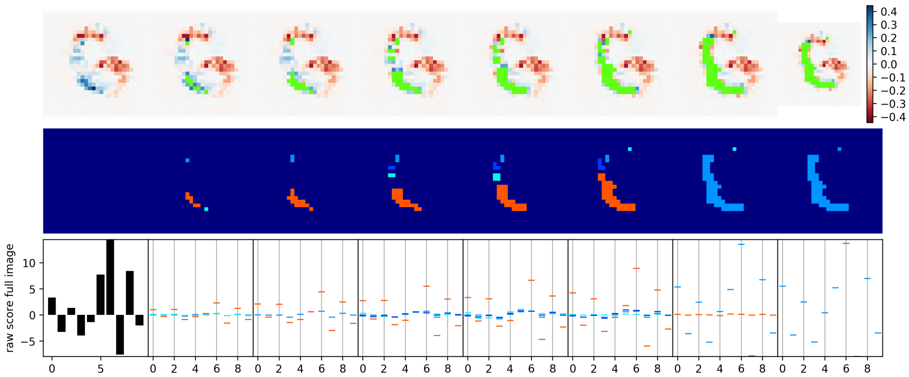
raw score full image

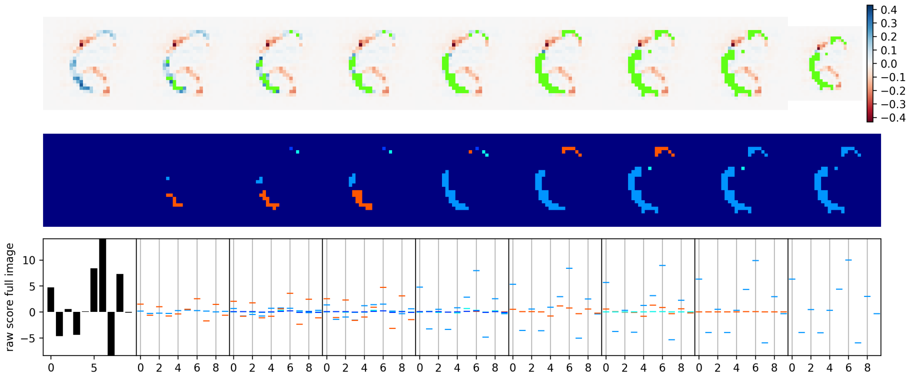
raw score full image

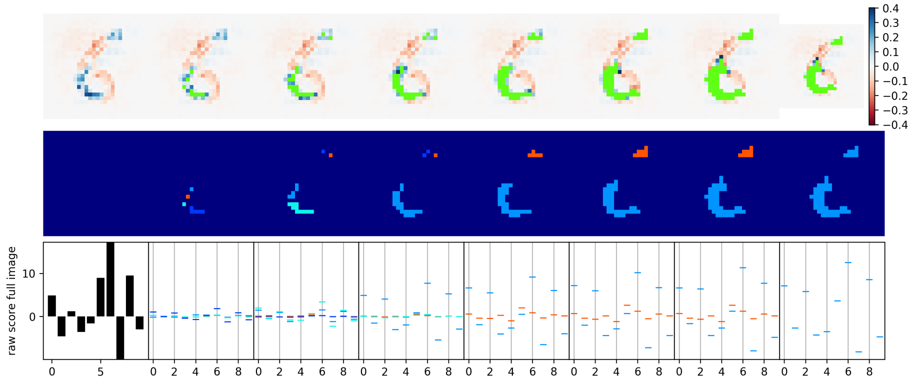


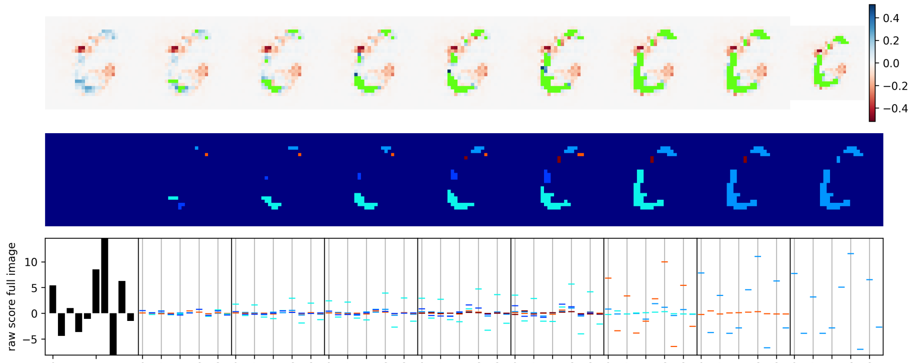


**MNIST lowest-predicted examples.** Here, the model used is the same as in Sec 4.3.2 and the interpretation of the figure produced is the same as in Fig 3.

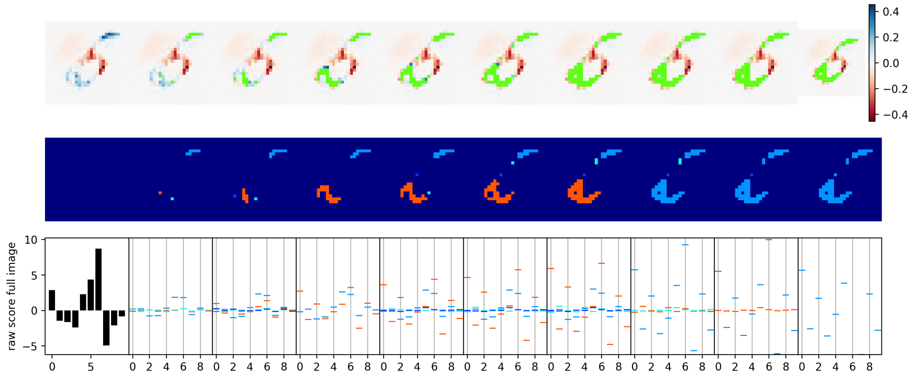

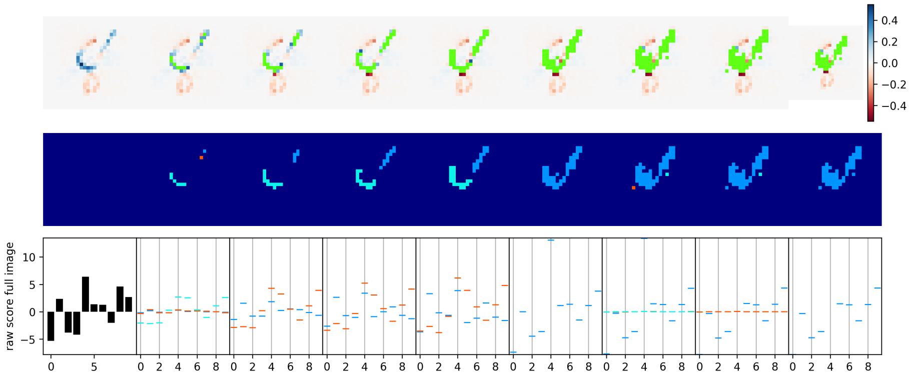


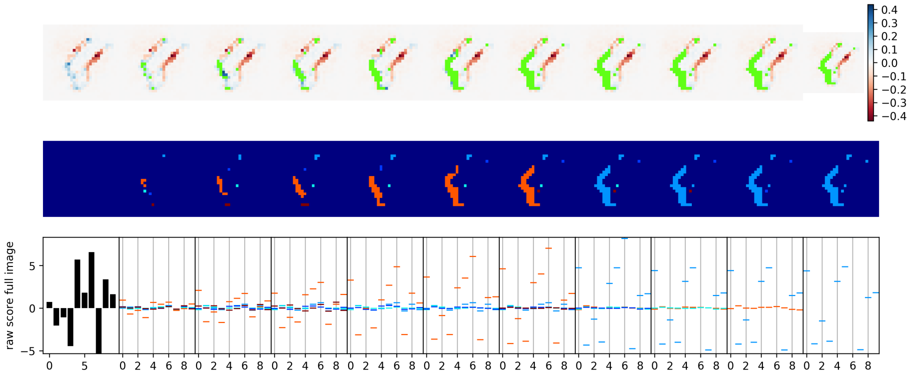


**Imagenet top-predicted examples.** Here, the model used and figure produced correspond to that in Fig 3.

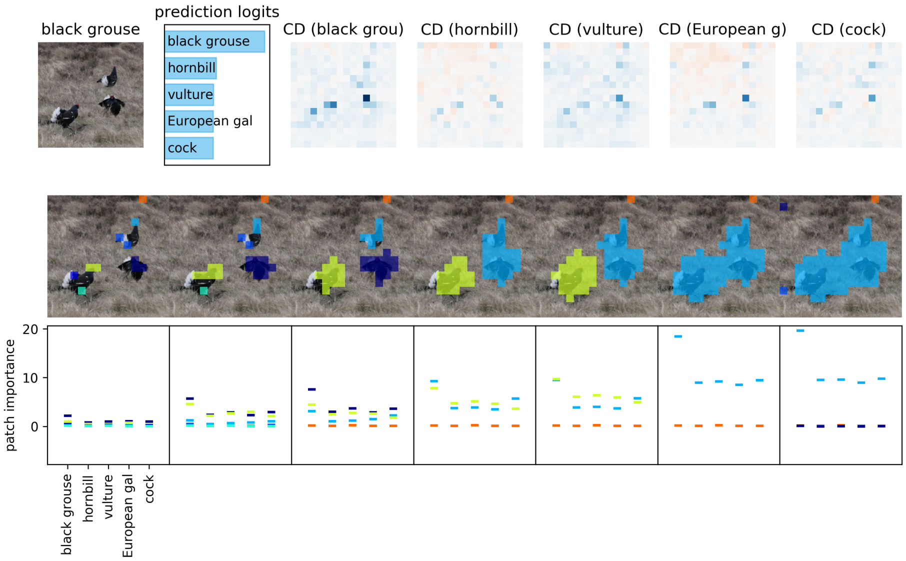
black grouse
prediction logits
black grouse
hornbill
vulture
European gal
cock
CD (black grou)
CD (hornbill)
CD (vulture)
CD (European g)
CD (cock)
patch importance
20
10
0
black grouse
hornbill
vulture
European gal
cock

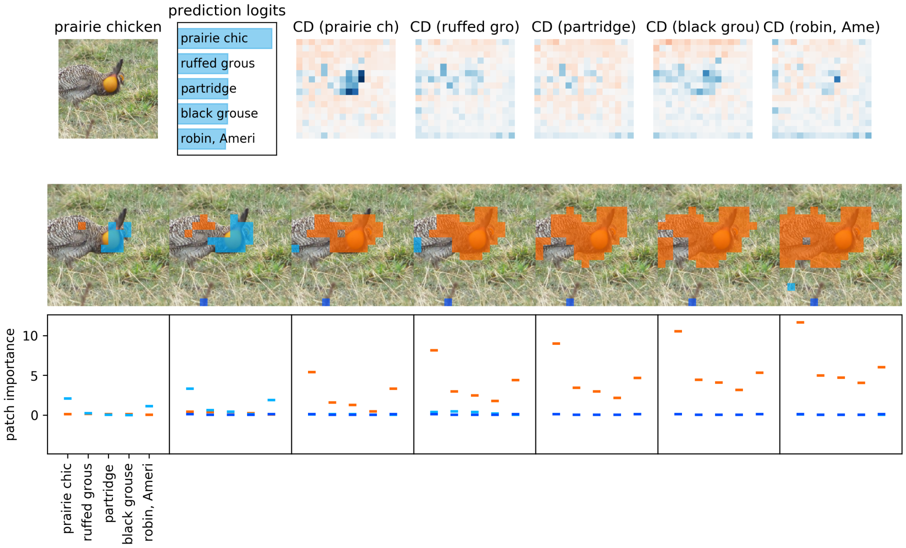
prairie chicken
prediction logits
prairie chic
ruffed grous
partridge
black grouse
robin, Ameri
CD (prairie ch)
CD (ruffed gro)
CD (partridge)
CD (black grou)
CD (robin, Ame)
patch importance
10
5
0
prairie chic
ruffed grous
partridge
black grouse
robin, Ameri

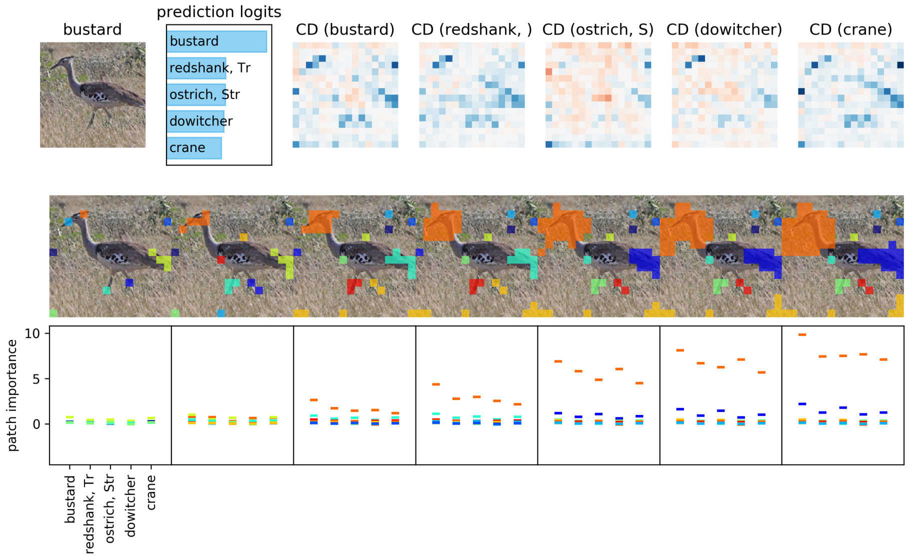


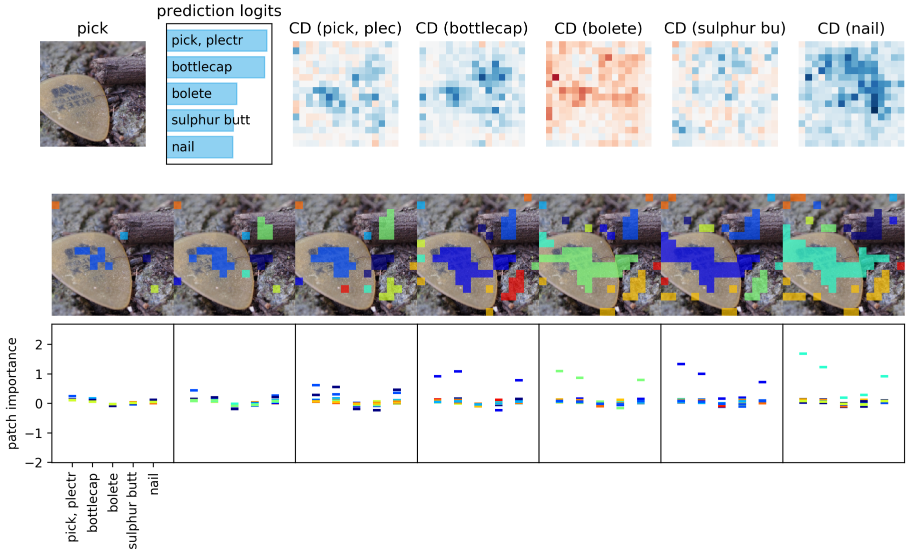


**Imagenet lowest-predicted examples.** Here, the model used and figure produced correspond to that in Fig **??**.

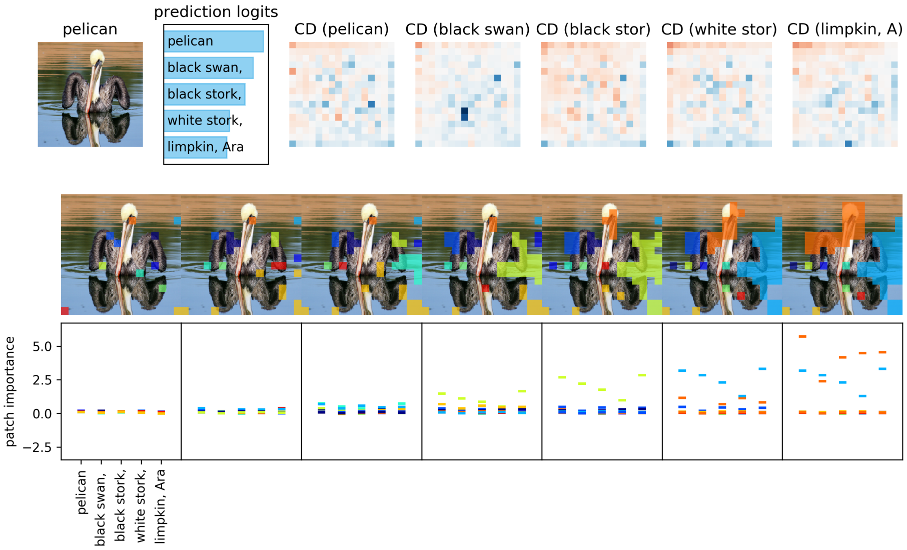
pelican
prediction logits
pelican
black swan,
black stork,
white stork,
limpkin, Ara
CD (pelican)
CD (black swan)
CD (black stor)
CD (white stor)
CD (limpkin, A)
patch importance
5.0
2.5
0.0
−2.5
pelican
black swan,
black stork,
white stork,
limpkin, Ara

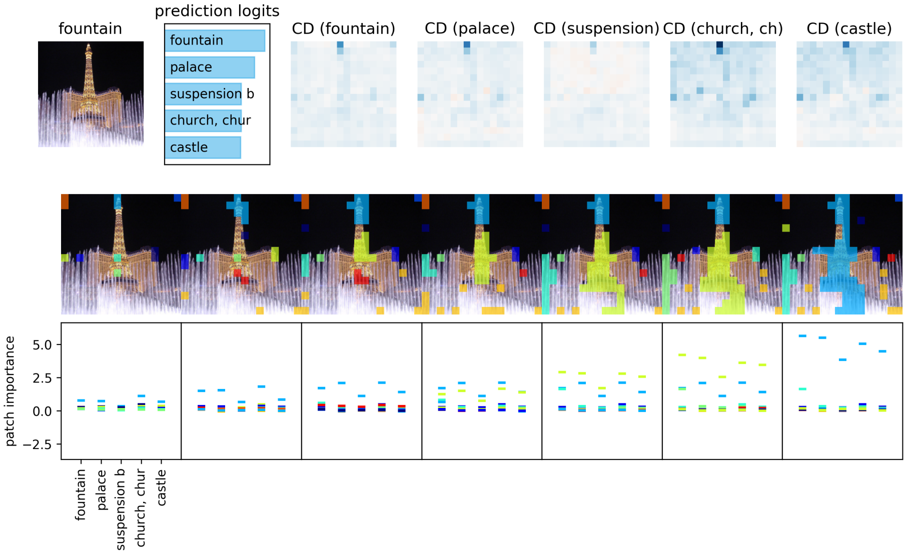
fountain
prediction logits
fountain
palace
suspension b
church, chur
castle
CD (fountain)
CD (palace)
CD (suspension)
CD (church, ch)
CD (castle)
patch importance
5.0
2.5
0.0
−2.5
fountain
palace
suspension b
church, chur
castle
